# Supplementary material for: C-FLAT: Control-FLow ATtestation for Embedded Systems Software
Source: arXiv:1605.07763 source file (2016-08-17)
Supplement: Supplementary file 1 [file appendix.tex]

\emph{Note that this section only serves as a reference for those text blocks that have 
significantly changed}

\section{Use-Case}
% Old Use-Case Model
The envisaged threat model, an example of which is shown in Figure~\ref{fig:use-case}, 
is based on the following scenario: the prover is an embedded system which directly 
connects to several sensors and actuators. This represents a typical set-up for 
devices such as a programmable logic controllers (PLCs) that connect to sensors and 
actuators that interface to the analog (physical) environment~\cite{field-device-security}. 
A user interface allows the verifier to execute commands on the prover's device (step~1). 
In our example, the prover offers two functions. The first,  
\texttt{function\_priv}, is privileged, e.g., it might allow the verifier to perform a software 
update. In contrast, \texttt{function\_A} allows the verifier to probe attached sensors 
which respond with input ($i_1,i_2$) in step~2 and~3. Based on the provided input, the prover 
executes \texttt{function\_A} (step~4).

\begin{figure}[htbp]
	\centering
		\includegraphics[width=\linewidth]{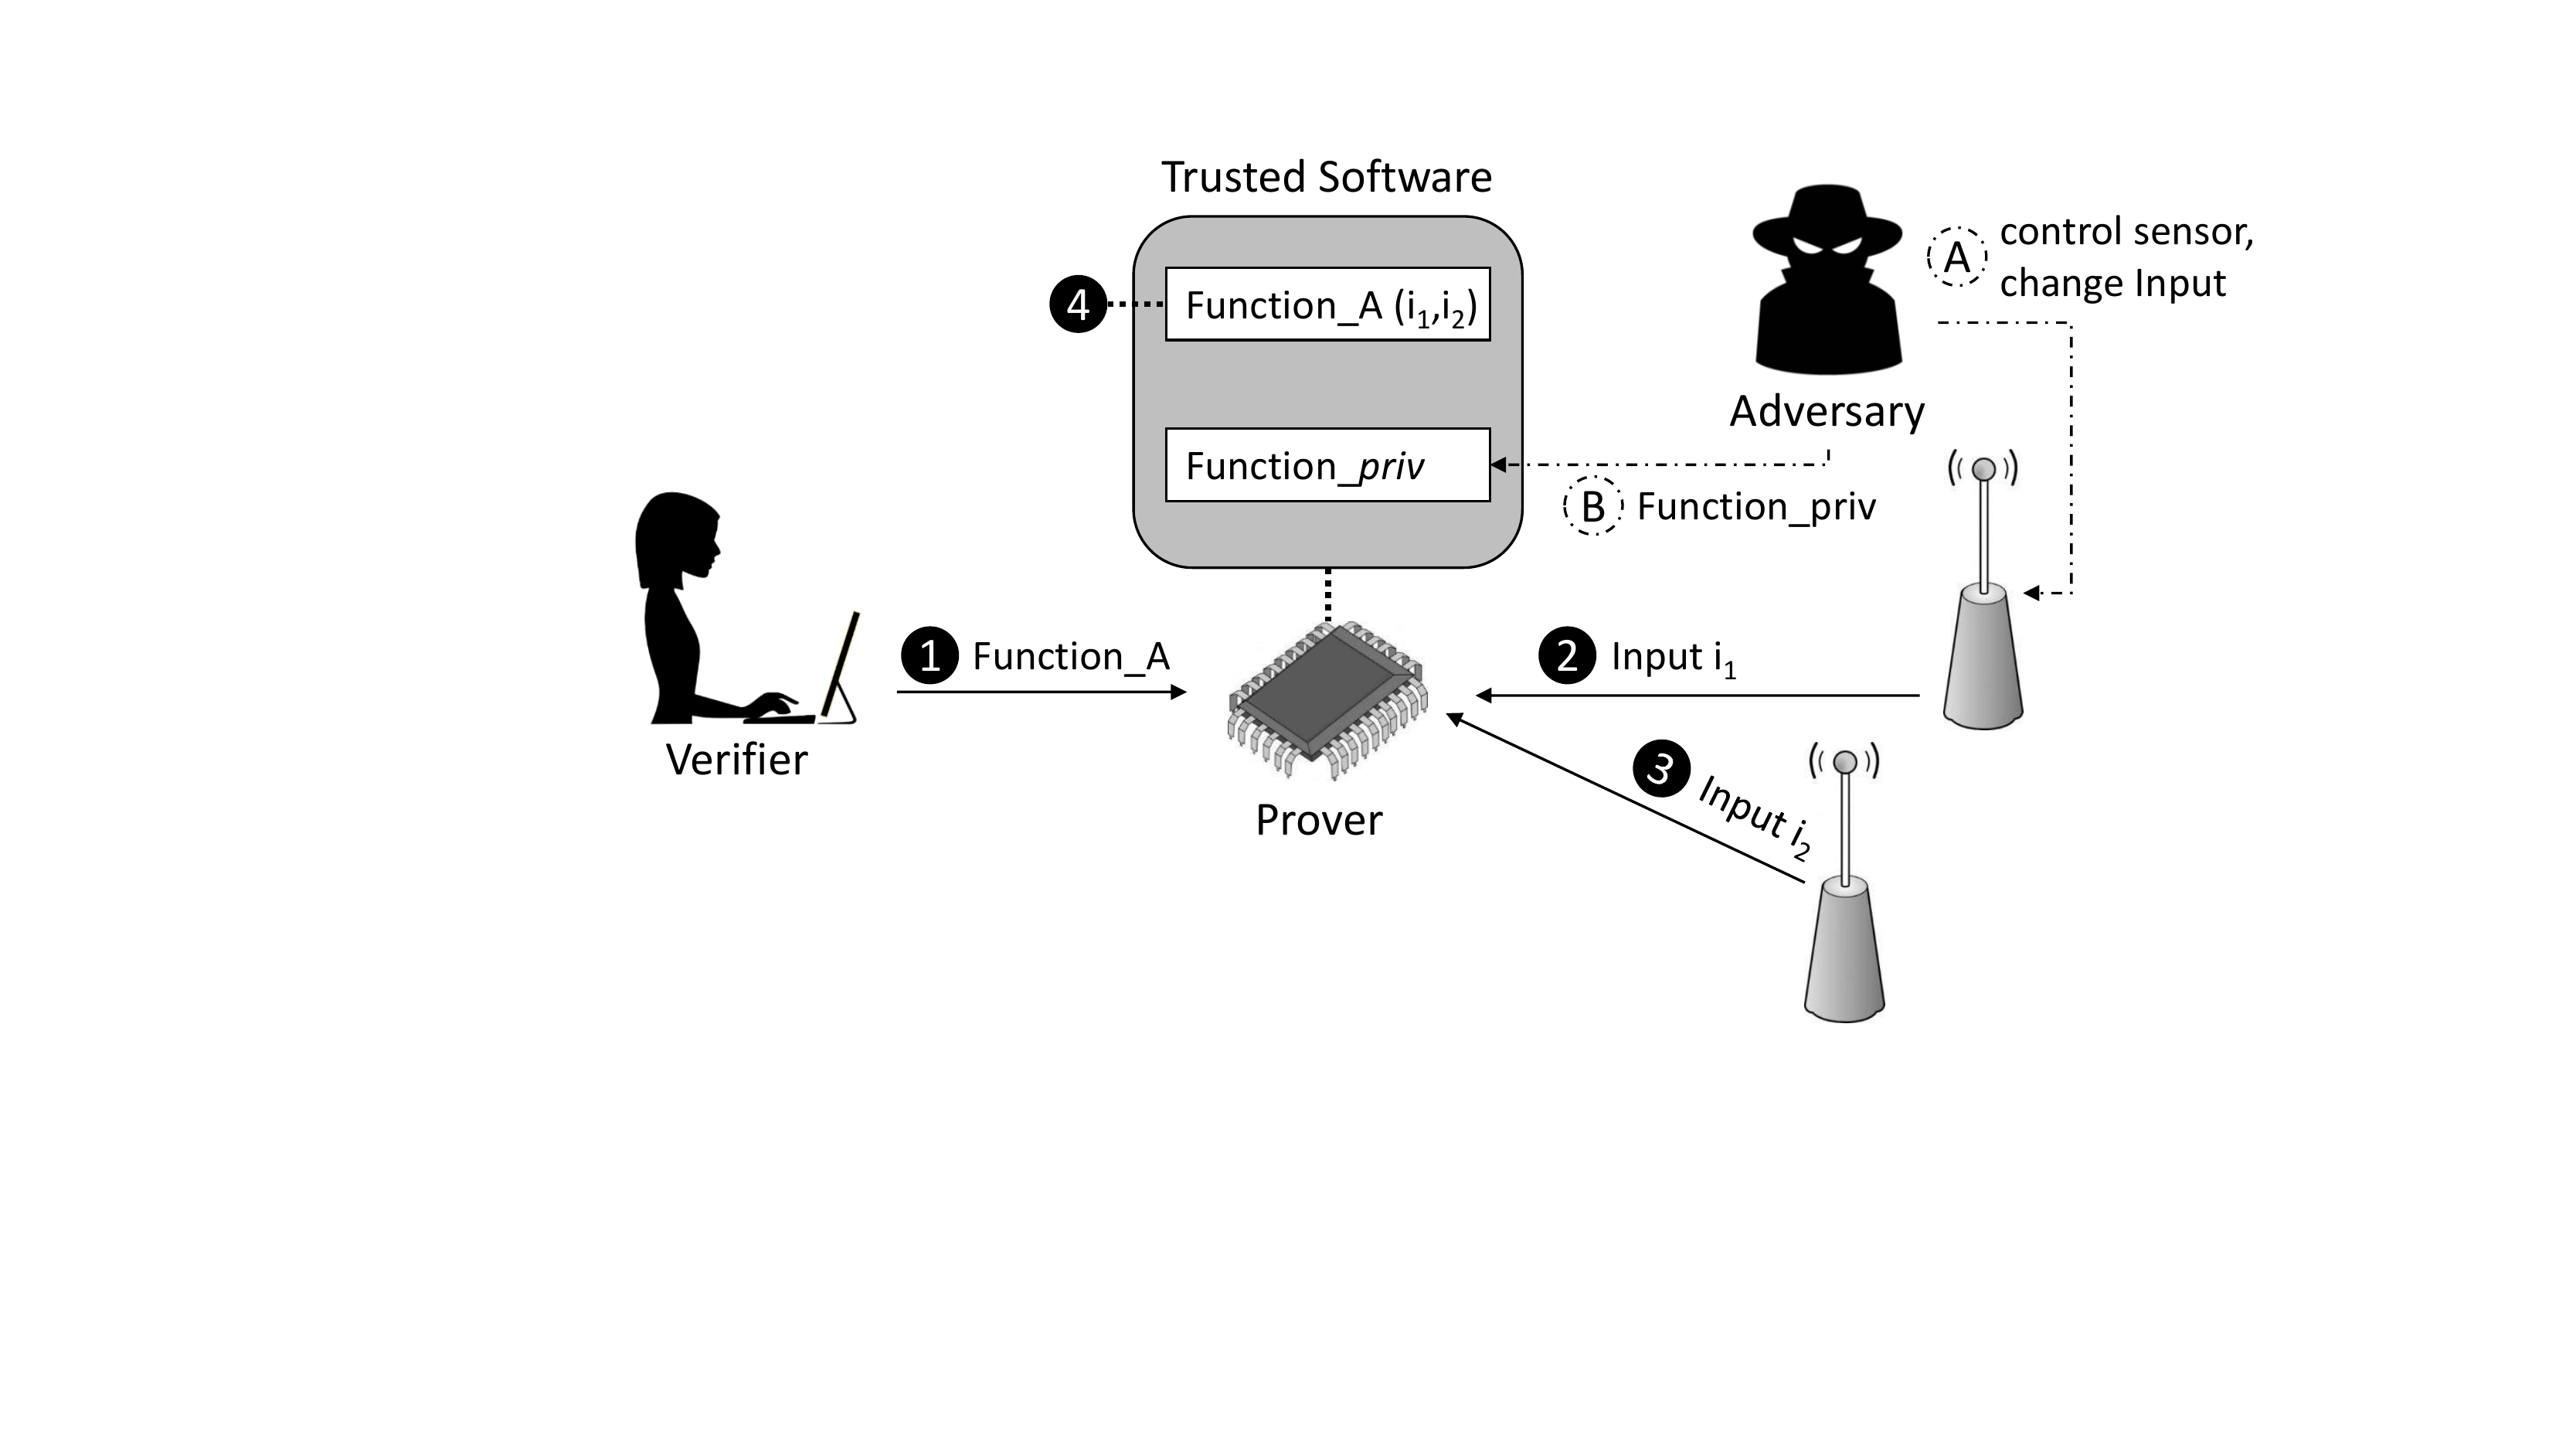}
	\caption{Use-case and threat model}
	\label{fig:use-case}
\end{figure}

\paragraph{Capabilities of Adversary}
We assume the adversary capable of fully subverting attached sensors and
producing arbitrary malicious inputs (step~A). However, we exclude the setting where
the adversary has direct (physical) control over the prover. Typical attestation methods 
ensure that only benign, trusted (yet vulnerable) software is executed on the prover. 
Thus, the adversary can only communicate with the prover by providing malicious inputs 
to the trusted software. In particular, the malicious input exploits a program bug to divert 
the program's control flow to \texttt{function\_priv} in order to install a new firmware (step~B). 

Our goal is to detect execution of malicious control flow paths on the prover within 
a runtime attestation protocol. In other words, we need to detect step~B in 
Figure~\ref{fig:use-case}.

%---------------------------------------------------
\section{Attestation Protocol} \label{sec:protocol}
%---------------------------------------------------
\noindent
Figure~\ref{fig:protocol} presents at high-level how our control-flow attestation mechanism 
is embedded into an attestation protocol. In order to perform the validation of the 
application's taken control flows, the verifier needs to compute the set of valid hash values 
$\left\{H_1...H_n \right\}$ and allowed loop iterations $\left\{|H_1|...|H_n|\right\}$ 
based on static analysis techniques. In general, these sets can be pre-computed 
before the attestation protocol starts. Alternatively, the verifier 
can calculate the hash values on-the-fly based on a random initialization value ($IV$) that is
provided as an input to the first hash measurement in \tool, i.e., $H_1(IV,2)$ in 
Figure~\ref{fig:use-case}. 

\begin{figure}[htbp]
	\centering
		\includegraphics[width=\linewidth]{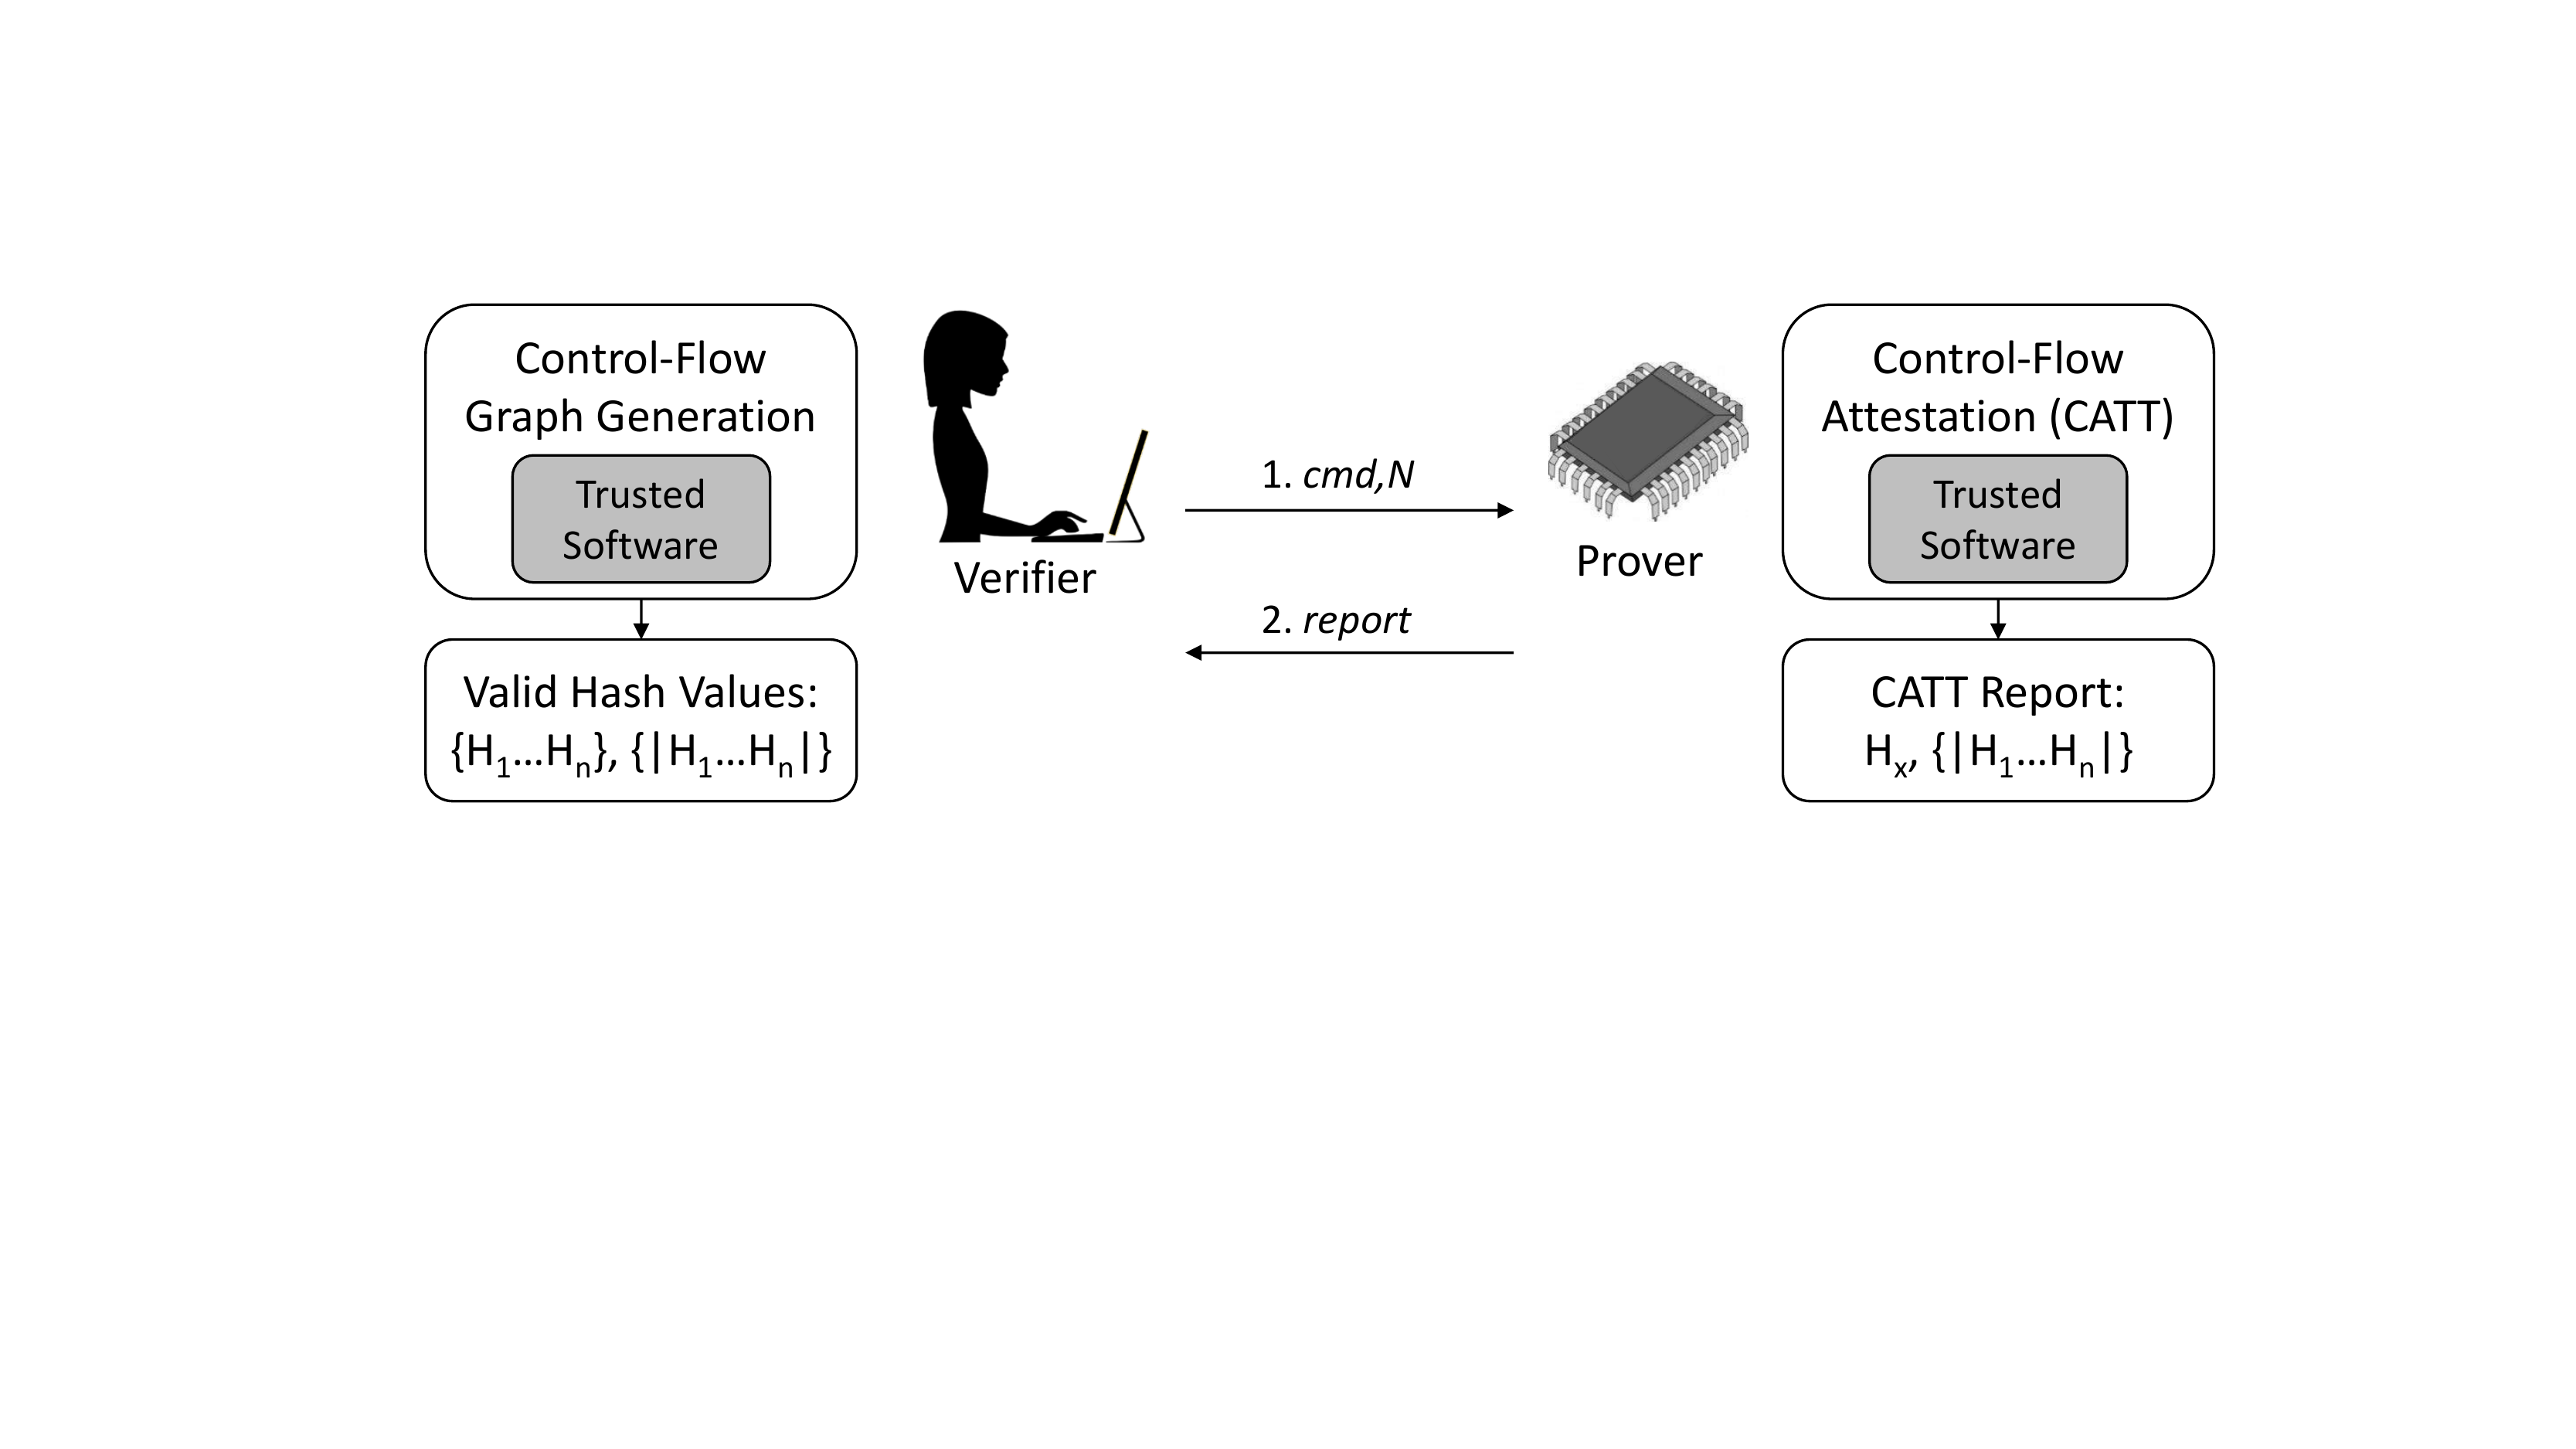}
	\caption{\tool\ attestation protocol}
	\label{fig:protocol}
\end{figure}

In the attestation protocol, the verifier first transmits the desired command (cmd) or function she desires 
to be executed on the prover's device and a nonce to ensure freshness. Subsequently, the 
prover executes the target command  under the supervision of \tool. That is, \tool\ builds the 
hash chain over the taken execution path. Finally, it sends the attestation report back to the 
verifier for verification. The verifier checks the freshness of the message and the attestation 
report based on the pre-computed hash sets. Similar to conventional attestation protocols, 
the prover's report should be embedded into a signed certificate. As mentioned in 
Section~\ref{sec:model}, we consider an adversary who cannot directly control the 
prover's device but only provide malicious inputs to the prover's trusted software. Further, 
the adversary cannot disable \tool\ to undermine runtime attestation. In 
Section~\ref{sec:future-strategies}, we elaborate on several implementation strategies that 
provide secure enforcement of the \tool\ measurement mechanism.
